# Supplementary material for: Violation of the Cauchy-Schwarz inequality with matter waves
Source: arXiv:1204.0058 source file (2012-06-27)
Supplement: Supplementary file 1 [file CS_PRL_Supplementary_resubmit_final.pdf]

Supplementary material for EPAPS

# Violation of the Cauchy-Schwarz inequality with matter waves

K. V. Kheruntsyan,* J.-C. Jaskula, P. Deuar, M. Bonneau, G. B. Partridge,
J. Ruaudel, R. Lopes, D. Boiron, and C. I. Westbrook
*To whom correspondence should be addressed; E-mail: karen.kheruntsyan@uq.edu.au

***Definitions of correlation functions.*** The second-order correlation function $\mathcal{G}^{(2)}(\mathbf{k},\mathbf{k}')$ between the particle number densities at two points in momentum space is defined as

$$\mathcal{G}^{(2)}(\mathbf{k},\mathbf{k}') = \langle :\hat{n}(\mathbf{k})\hat{n}(\mathbf{k}'): \rangle = \langle \hat{a}^\dagger(\mathbf{k})\hat{a}^\dagger(\mathbf{k}')\hat{a}(\mathbf{k}')\hat{a}(\mathbf{k})\rangle. \quad \text{(S1)}$$

Here, $\hat{a}(\mathbf{k})$ is the Fourier transform of the atomic field annihilation operator $\hat{\Psi}(\mathbf{x})$, and $\hat{n}(\mathbf{k}) = \hat{a}^\dagger(\mathbf{k})\hat{a}(\mathbf{k})$ is the density operator corresponding to the atomic momentum distribution (with $\mathbf{k}$ denoting the wave-vector $\mathbf{k} = m\mathbf{v}/\hbar$).

The normalized correlation functions shown in Fig. 2 of the main text are defined as

$$g^{(2)}_{\rm BB}(\Delta\mathbf{k}) = \mathcal{G}^{(2)}_{\rm BB}(\Delta\mathbf{k}) \Big/ \int_{\mathcal{V}} d^3\mathbf{k}\, \langle\hat{n}(\mathbf{k})\rangle\langle\hat{n}(-\mathbf{k}+\Delta\mathbf{k})\rangle, \quad \text{(S2)}$$

and

$$g^{(2)}_{\rm CL}(\Delta\mathbf{k}) = \mathcal{G}^{(2)}_{\rm CL}(\Delta\mathbf{k}) \Big/ \int_{\mathcal{V}} d^3\mathbf{k}\, \langle\hat{n}(\mathbf{k})\rangle\langle\hat{n}(\mathbf{k}+\Delta\mathbf{k})\rangle. \quad \text{(S3)}$$

The normalization ensures that for uncorrelated densities $g^{(2)}_{\rm BB}(\Delta\mathbf{k}) = 1$ and $g^{(2)}_{\rm CL}(\Delta\mathbf{k}) = 1$.

These functions are shown in Fig. 2 of the main text. The widths and amplitudes of the BB and CL correlation functions are measured using Gaussian fits to their cuts through the centre of the 2D surface plots along the $k_z$ and $k_{xy}$ axis; the fits and the data are shown in Fig. S1 (same data as in Fig. 2 of the main text but with error bars).

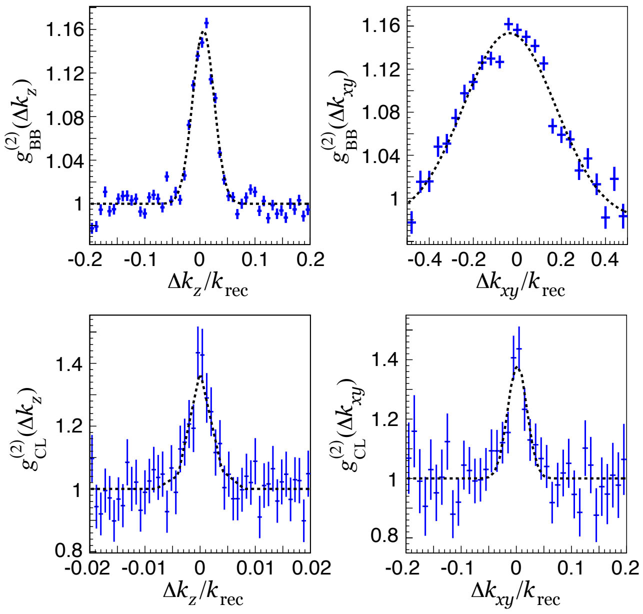


Figure S 1. Central cuts of the BB and CL correlation functions, $g^{(2)}_{\rm BB}(\Delta\mathbf{k})$ and $g^{(2)}_{\rm CL}(\Delta\mathbf{k})$, along the $k_z$ and $k_{xy}$ axis.

***CS violation and correlation widths.*** A fair understanding of the dependence of the multimode CS violation $C$ on the correlation functions can be gained from a simple model, which is readily related to the experimental data. Let us make several assumptions: (A) a Gaussian shape for the normalized correlation functions (those shown in Fig. 2 of the main text):

$$g^{(2)}_{\rm CL/BB}(\Delta\mathbf{k}) = 1 + h_{\rm CL/BB}\prod_d e^{-\Delta k_d^2/2\sigma^2_{{\rm CL/BB},d}}, \quad \text{(S4)}$$

where $CL$ and $BB$ are the two kinds of correlations, the index $d = x, y, z$ runs over spatial directions, $\sigma_{{\rm CL/BB},d}$ are standard deviations (correlation lengths, in wave-number units) of the correlation peak, and $h_{\rm CL/BB}$ are the peak heights above the background level of unity. Let us further assume (B) that the counting zones $\mathcal{V}_i$ are much broader than the relevant correlation lengths in all directions. This allows us to neglect boundary effects caused by atom pairs in which one member lies just inside the zone and the other just outside [1]. Finally, for simplicity we assume (C) that the halo density in the relevant regions is constant: $\langle\hat{n}(\mathbf{k}+\mathbf{\Delta k})\rangle = \bar{n}$, and (D) that the two counting zones have the same widths in each direction $d$, hence the same overall momentum-space volumes $\mathcal{V}_1 = \mathcal{V}_2 \equiv \mathcal{V}$.

With these assumptions, the integrated correlation functions are

$$\overline{\mathcal{G}}^{(2)}_{ii} \approx \bar{n}^2\mathcal{V}\left\{\mathcal{V} + h_{\rm CL}(2\pi)^{3/2}\prod_d \sigma_{{\rm CL},d}\right\} \quad \text{(S5)}$$

$(i = 1, 2)$ and

$$\overline{\mathcal{G}}^{(2)}_{12} \approx \bar{n}^2\mathcal{V}\left\{\mathcal{V} + h_{\rm BB}(2\pi)^{3/2}\prod_d \sigma_{{\rm BB},d}\right\}, \quad \text{(S6)}$$

where the counting zones $\mathcal{V}_1$ and $\mathcal{V}_2$ are non-overlapping. Taking the widths of the counting zones $\mathcal{V}$ as $L_d$, the next order corrections are $\sim \mathcal{O}(\sum_d \frac{\sigma_{{\rm CL/BB},d}}{L_d})$ with respect to the terms proportional to $h_{\rm CL/BB}$, and so are negligible due to our assumption (B).

It is useful to define an effective geometric mean correlation width

$$\bar{\sigma}^3_{\rm CL/BB} = \prod_d \sigma_{{\rm CL/BB},d}. \tag{S7}$$

The large counting volume assumption (B) means $\bar{\sigma}_{\rm CL/BB}/\mathcal{V}^{1/3} \ll 1$, and taking leading order terms in this small parameter, we use Eqs. (S5–S6) to obtain an estimate for the CS violation between opposite zones:

$$C \approx 1 + \frac{(2\pi)^{3/2}}{\mathcal{V}}\left[h_{\rm BB}\,\bar{\sigma}^3_{\rm BB} - h_{\rm CL}\,\bar{\sigma}^3_{\rm CL}\right]. \tag{S8}$$

Now it is clear that nonclassical measurements ($C > 1$) can still occur for a back-to-back correlation peak lower than the collinear one, provided that the coherence volume for the back-to-back pairs is correspondingly larger and that it still fits inside our counting volumes $\mathcal{V}$. Expression (S8) also hints that a maximally large CS violation will occur when the counting volumes are of about the same size as the coherence volumes, since the excursion above one is proportional to the ratios $\bar{\sigma}^3_{\rm CL/BB}/\mathcal{V}$.

***CS violation and the number of zones $M$.*** To apply the above model to our experiment, we take the radial ($r$) width of the counting zone $L_r$ to be approximately equal to the width $w_r$ of the scattering sphere in the radial direction, $L_r \approx w_r$. Also, the zone size is $L_z = k_{\rm rec}/8$ in the longitudinal $z$ direction (where we recall that the analyzed part of the scattering sphere corresponds to $|k_z| < 0.5k_{\rm rec}$, which is further cut into 8 polar zones), and $L_c \approx 2\pi k_{\rm rec}/(M/8)$ along the circumference of the ring in the $xy$ plane. With this,

$$C \approx 1 + M\,\frac{\sqrt{2\pi}}{w_r k^2_{\rm rec}}\left[h_{\rm BB}\,\bar{\sigma}^3_{\rm BB} - h_{\rm CL}\,\bar{\sigma}^3_{\rm CL}\right] \tag{S9}$$

This is a linear growth with $M$.

The width of a single zone along the circumference, $L_c$, becomes comparable with, or narrower than, the measured correlation width $\sigma_{{\rm BB},xy} \approx 0.21k_{\rm rec}$ when $M \gtrsim 150$. This is indeed when we start to see a deviation from the linear behaviour in Fig. 3 of the main text.

For large $M$, the zones are narrow along the circumference, so that the broad zone assumption (B) does not hold, and variation of $\Delta\mathbf{k}$ along this direction does not change the correlation from its peak value. If one carries out the calculation again, but with an alternative assumption (B′) that the counting zone is now much *narrower* than the correlation widths $\sigma_{{\rm CL/BB},d}$, the estimate of $C$ becomes

$$C \approx 1 + \frac{32\pi}{w_r k_{\rm rec}}\left[h_{\rm BB}\,\sigma_{{\rm BB},z}\,\sigma_{{\rm BB},xy} - h_{\rm CL}\,\sigma_{{\rm CL},z}\,\sigma_{{\rm CL},xy}\right], \tag{S10}$$

which amounts to a replacement of one set of Gaussian widths $\sigma_{{\rm CL/BB},xy}$ by $L_c/\sqrt{2\pi}$. The correlation coefficient $C$ reaches a saturation value that does not depend on $M$ at all, but may be larger or smaller than unity, depending on how the widths and heights play out. In our case it is still a violation, with $C > 1$.

If the zones $\mathcal{V}$ were made narrower in all directions than the corresponding correlation widths, we would recover the two-mode expression

$$C \approx \frac{h_{\rm BB}+1}{h_{\rm CL}+1}. \tag{S11}$$

In our case, since $h_{\rm BB} < h_{\rm CL}$, this would not be a CS violation anymore.

Finally, when one considers non-opposite zones, such as the lower experimental data in Fig. 3 of the main text, the value of $h_{\rm BB}$ tends to zero as there is no pairing. In this case, the expressions (S9) and (S10) show that $C$ will lie always slightly below unity for large counting zones. For the small-counting-zone limit, $C \to 1/g^{(2)}_{\rm CL}(0)$. In neither case can there be CS violation.

***Stochastic Bogoliubov simulations.*** The theoretical results shown in Fig. 3 of the main text come from numerical simulations using the positive-$P$ Bogoliubov method, which is described in detail in Ref. [2]. It was used previously for our experiment in Refs. [1, 3]. In a nutshell, we evolve the system in a time-dependent Bogoliubov approximation, taking the condensate part at time $t$ as the solution of the Gross-Pitaevskii mean field evolution equation for the colliding condensates. The numerical lattice required to describe this model is too large for a direct solution of the Bogoliubov-de Gennes equations to be tractable, so the fluctuation field (which is responsible for the scattered halo) is represented instead using the positive-$P$ representation. This leads to coupled linear stochastic differential equations which *can* be integrated numerically. The ensemble of such stochastic realisations corresponds to the full Bogoliubov dynamics, and allows one to estimate observables to within a well defined statistical accuracy.

Simulations were carried out for a collision of metastable $^4$He$^*$ atoms in the $m_F = 0$ state (with the $s$-wave scattering length of $a = 5.3$ nm) for several initial total number of atoms, $N = 50\,000$, $85\,000$, and $110\,000$ (the actual value in the experiment fluctuates from shot to shot in the vicinity of $\sim 10^5$). The atoms were assumed to be trapped initially in the $m_F = 1$ state in a harmonic trapping potential with frequencies $\omega_z/2\pi = 7.5$ Hz and $\omega_x/2\pi = \omega_y/2\pi = 1500$ Hz.

To begin with, several initial states were tried: a zero-temperature ($T = 0$) Bose-Einstein condensate (BEC), and $T > 0$ quasicondensates in elongated 3D traps with phase coherence lengths of $l_\phi = 45$ $\mu$m and $l_\phi = 100$ $\mu$m (taken as a half-width-at-half-maximum of the first-order correlation function $g^{(1)}(0, z)$ from the center of the trap in the longitudinal direction), which are in the range expected for the cloud in the experiment. For comparison, the longitudinal size of the initial cloud along $z$ is about 980 $\mu$m.

The magnitude of the calculated $C$ at long times differed by at most 0.007 between the simulations with quasicondensate and BEC initial conditions (see Fig. S2). Since this is a

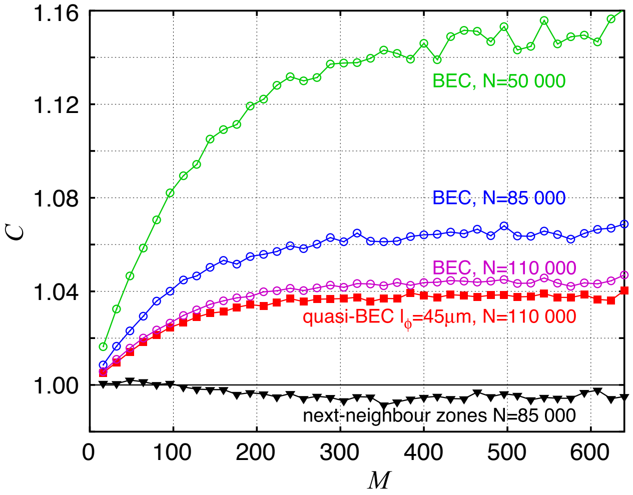


Figure S2. Calculated correlation coefficient $C$ as a function of the number of zones $M$ at the end of the simulation ($t = 186$ $\mu$s for the $N = 110\,000$ atom simulations, 248 $\mu$s for the others). Circles are for $C$ between opposite zones and BEC initial conditions; squares similarly, but with a quasicondensate initial condition having the shortest phase coherence length $l_\phi = 45$ $\mu$m. Filled triangles show $C$ between next-neighbour zones, which do not violate the CS inequality ($C < 1$), as expected. One sees that the value of $C$ depends strongly on $N$, while its shape as a function of $M$ is almost unchanged.

very small effect on $C$ in comparison with the effect of particle number (or in comparison with the effect on the shape of correlation functions), we will consider mainly the BEC initial conditions in what follows. The simulation of quasicondensates with a Bogoliubov description, in which the initial $T > 0$ states were based on the description of Petrov *et al.* [4] for elongated 3D clouds, will be described in a future work [5].

***Theoretical predictions for*** $C$. The simulation data in Fig. 3 of the main text are for a time of 248 $\mu$s after the start of the collision with 85 000 atoms, which we regard as the best-fit value of $N$.

The values of the correlation coefficient at the end of simulations for various atom numbers and initial conditions are shown in Fig. S2. The time evolution of its saturation value at large $M$ [i.e., small counting volumes as per Eq. (S10)] is shown in Fig. S3(b), along with the time evolution of the overall number of scattered atoms [Fig. S3(a)]. It is seen that the magnitude of $C$ depends strongly on the initial number of atoms $N$, while its shape as a function of $M$ remains almost unchanged. In particular, small $N$ and hence small number of scattered particles in the halo, $N_{sc}$ [see Fig. S3(a)] correspond to large values of $C$ for a given counting zone size. This can be roughly understood from a simple two-mode model of standard spontaneous parametric down-conversion in the undepleted pump approximation [6], with a Hamiltonian $\hat{H} \sim \hat{a}_1^\dagger \hat{a}_2^\dagger + \mathrm{h.c.}$ that produces atom pairs in the $a_1$ and

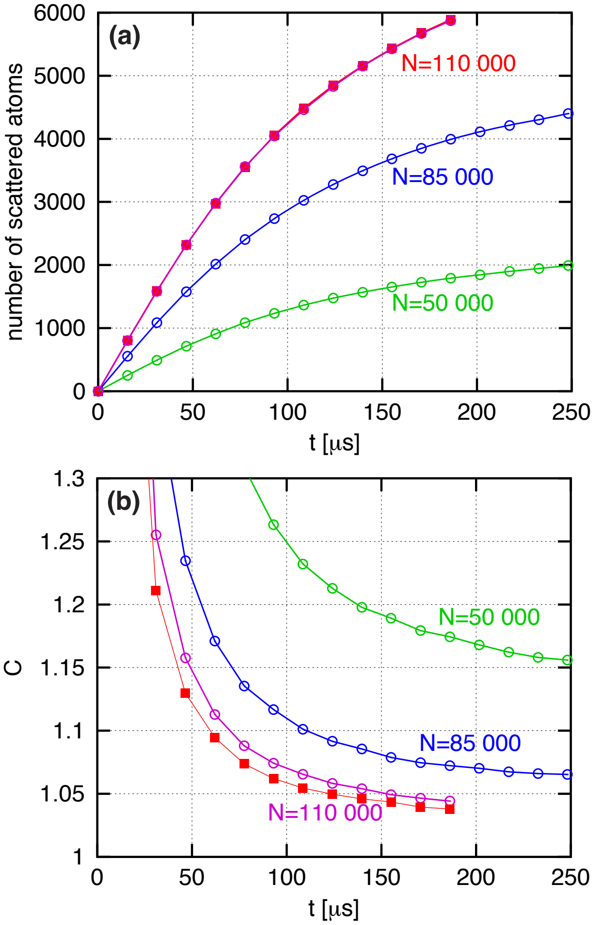


Figure S3. Calculated time evolution. Panel (a) shows the number of scattered atoms as a function of time for various initial atom numbers $N$. Panel (b) shows the saturation mean value of $C$ at large $M$ between opposite zones – the value is averaged over $M \geq 400$. In both panels, circles are for BEC initial conditions, squares for the $l_\phi = 45$ $\mu$m quasicondensate as in Fig. S2. The $C(M)$ data in Fig. 3 of the main text and in Fig. S2 here are for the last times shown here. One sees that at that moment $C$ has already achieved its long-time value, or is very close to it.

$a_2$ modes. This is a process similar to the one that occurs during our condensate collision. In this toy model, the BB correlation analogue is $g_{12}^{(2)} = 2 + 1/n$ [7], where $n$ is the mean particle number in modes $a_1$ and $a_2$ ($n_1 = n_2 \equiv n$), and the CL correlation analogue is $g_{11}^{(2)} = g_{22}^{(2)} = 2$. Hence, $C \approx 1 + 1/2n$ in this model, showing a similar scaling with atom number to our simulations. Resorting to this toy model is done only for qualitative understanding of the scaling of $C$ with $N_{sc}$ and hence with the number of atoms in a given counting zone. The quantitative aspects of the model, however, are too crude to be applicable to our system due to the rapid changes in the "pump" (source condensate) density profile, which is in sharp contrast to the undepleted, i.e., *constant* in time, pump approximation.

The experimental values in Fig. 3 of the main text come from an average over many realizations with different atom

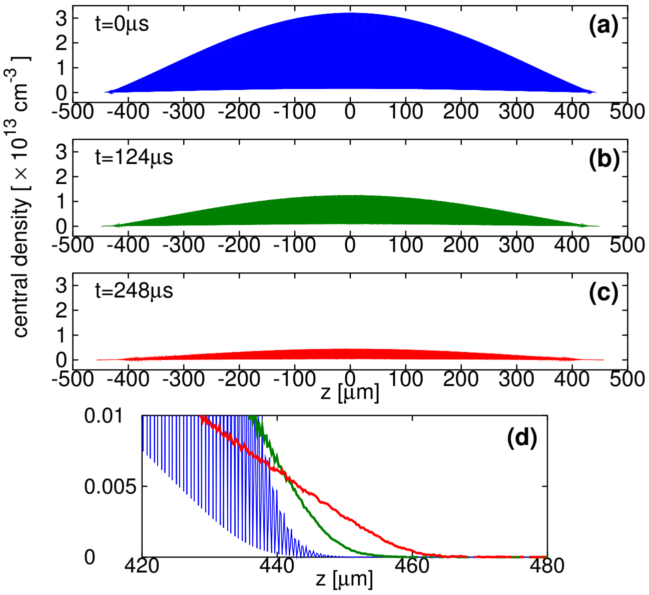


Figure S 4. Central density along $z$ (at $x = y = 0$) of the two colliding condensates, for the total initial number of atoms $N = 85,000$, shown at three different times: $t = 0$ – (a), $t = 124\,\mu$s – (b), and $t = 248$ $\mu$s – (c). The overlap region includes the interference fringes, which are, however, not visible on this scale due to the high frequency of the modulation. As we see, the peak density at $t = 248$ $\mu$s is reduced by a factor of $\sim 7$ due to the rapid expansion of the condensates in the transverse dimensions, which is the main reason for the collision to cease. Panel (d) shows detail at the cloud edges.

numbers $N$ from shot to shot. However, the contribution of small-atom-number shots (which would have a high magnitude of $C$, and poor signal-to-noise) to the atom-number fluctuations that go into the calculation of $C$ is small. Taking this into account, and noting that $N \approx 85\,000$ is the most typical value, best agreement between this value and experiment is very reasonable.

The time evolution in Fig. S3 shows that, at the final simulation times shown in Fig. 3 of the main text and Fig. S3 here, the correlation coefficient $C$ is already at, or very close to, its long-time value. The maximum simulation time is the result of a trade-off between computational efficiency and accuracy — the size of the numerical grid required to encompass the clouds grows rapidly with longer times. Even though our maximum simulation time is appreciably shorter than the time it takes for the clouds to move completely past each other along $z$ (about 5 ms), the production of halo particles is already strongly saturating by the end of the simulation [see Fig. S3(a)]. This is due to a rapid loss of central density of the colliding source BECs because of their expansion perpendicular to the long (collision) axis. In other words, the end of collision and the saturation in the number of scattered atoms in Fig. S3(a) is determined not by a geometric consideration (i.e., a complete spatial separation of the colliding BECs along $z$), but by the rapid loss of peak density (see Fig. S4) due to the expansion in the transverse direction. The pair production rate is roughly proportional to the integral of density squared [8], which is the reason for the premature cessation of particle scattering, and allows relatively short simulation times to be considered adequate.

***Cauchy-Schwarz inequality and sub-Poissonian number imbalance.*** The strength of correlation between the atom number fluctuations in two diametrically opposite zones on the collision halo can also be characterised via a normalised variance [1]

$$V = \frac{\langle[\Delta(\hat{N}_1 - \hat{N}_2)]^2\rangle}{\langle\hat{N}_1\rangle + \langle\hat{N}_2\rangle}, \quad \text{(S12)}$$

which can be rewritten in terms of the second-order correlation functions,

$$V = 1 + \frac{\overline{\mathcal{G}}^{(2)}_{11} + \overline{\mathcal{G}}^{(2)}_{22} - 2\overline{\mathcal{G}}^{(2)}_{12} - (\langle\hat{N}_1\rangle - \langle\hat{N}_2\rangle)^2}{\langle\hat{N}_1\rangle + \langle\hat{N}_2\rangle}. \quad \text{(S13)}$$

The variance is normalised to the level of uncorrelated, Poissonian fluctuations and $V < 1$ implies sub-Poissonian statistics of the relative number imbalance. From this we see that the relationship between sub-Poissonian number imbalance and the violation of the CS inequality is especially transparent in the symmetric case of $\langle\hat{N}_1\rangle = \langle\hat{N}_2\rangle$, in which case stronger-than-classical correlation, $\overline{\mathcal{G}}^{(2)}_{12} > [\overline{\mathcal{G}}^{(2)}_{11}\overline{\mathcal{G}}^{(2)}_{22}]^{1/2}$ (in the sense of CS violation), follows from $V < 1$ and hence represents a necessary condition for sub-Poissonian statistics. This last assertion follows from the fact that, if $V < 1$ and $\langle\hat{N}_1\rangle = \langle\hat{N}_2\rangle$, then one must have $\overline{\mathcal{G}}^{(2)}_{12} > \frac{1}{2}(\overline{\mathcal{G}}^{(2)}_{11} + \overline{\mathcal{G}}^{(2)}_{22})$, where $\frac{1}{2}(\overline{\mathcal{G}}^{(2)}_{11} + \overline{\mathcal{G}}^{(2)}_{22}) \geq [\overline{\mathcal{G}}^{(2)}_{11}\overline{\mathcal{G}}^{(2)}_{22}]^{1/2}$, and therefore $\overline{\mathcal{G}}^{(2)}_{12} \geq [\overline{\mathcal{G}}^{(2)}_{11}\overline{\mathcal{G}}^{(2)}_{22}]^{1/2}$. The opposite is, however, not true in general, because having $\overline{\mathcal{G}}^{(2)}_{12} > [\overline{\mathcal{G}}^{(2)}_{11}\overline{\mathcal{G}}^{(2)}_{22}]^{1/2}$ does not necessarily guarantee $V < 1$, unless $\overline{\mathcal{G}}^{(2)}_{11} = \overline{\mathcal{G}}^{(2)}_{22}$. Thus, violation of the CS inequality and sub-Poissonian number imbalance are equivalent only in the completely symmetric case of $\langle\hat{N}_1\rangle = \langle\hat{N}_2\rangle$ and $\overline{\mathcal{G}}^{(2)}_{11} = \overline{\mathcal{G}}^{(2)}_{22}$.

We emphasise, however, that the equivalence of the CS violation and the relative number imbalance in the symmetric case (or the expected 'approximate equivalence' in the nearly symmetric case, as is the case in our experiment) is only of qualitative nature. The quantitative relationship between the *strength* of the CS violation and the *degree* of suppression of $V$ below the Poissonian level of fluctuations can, on the other hand, be very different if we analyse these as functions of the zone size or the number of zones $M$ into which we cut the scattering halo. Indeed, as was demonstrated in Ref. [1], strong suppression of $V$ below unity is observed for the broader zones (see Fig. 3 of [1]) – a situation in which the CS inequality is only marginally violated as seen from Fig. 3 of the main text at small $M$. Conversely, the CS inequality is maximally violated for large $M$ (smaller zone sizes), in which case the variance $V$ is almost indistinguishable from the Poissonian shot-noise level of $V = 1$. This difference highlights

the importance of quantifying any particular type of quantum correlations in an operationally defined manner.


[1] J.-C. Jaskula, M. Bonneau, G. B. Partridge, V. Krachmalnicoff, P. Deuar, K. V. Kheruntsyan, D. Boiron, A. Aspect, and C. I. Westbrook, Phys. Rev. Lett. **105**, 190402 (2010).

[2] P. Deuar, J. Chwedeńczuk, M. Trippenbach, and P. Ziń, Phys. Rev. A **83**, 063625 (2011).

[3] V. Krachmalnicoff, J.-C. Jaskula, M. Bonneau, V. Leung, G. B. Partridge, D. Boiron, C. I. Westbrook, P. Deuar, P. Ziń, M. Trippenbach, and K. V. Kheruntsyan, Phys. Rev. Lett. **104**, 150402 (2010).

[4] D. S. Petrov, G. V. Shlyapnikov, and J. T. M. Walraven, Phys. Rev. Lett. **87**, 050404 (2001).

[5] P. Deuar *et al.*, in preparation.

[6] D. F. Walls and G. J. Milburn, *Quantum Optics*, 2nd ed. (Springer, Berlin, 2008).

[7] C. M. Savage, P. E. Schwenn, and K. V. Kheruntsyan, Phys. Rev. A **74**, 033620 (2006).

[8] A. Perrin, C. M. Savage, D. Boiron, V. Krachmalnicoff, C. I. Westbrook, and K. V. Kheruntsyan, New J. Phys. **10**, 045021 (2008).
